# Supplementary material for: Bayesian Pose Graph Optimization via Bingham Distributions and Tempered Geodesic MCMC
Source: arXiv:1805.12279 source file (2019-03-30)
Supplement: Supplementary file 1 [file appendix.tex]

\appendix

\input{expmap}
\input{analysis}
\input{gradients}
\input{supp-experiments}
